# Supplementary material for: Identifying Non-Control Security-Critical Data through Program Dependence Learning
Source: arXiv:2108.12071 source file (2024-05-01)
Supplement: Supplementary file 1 [file appendix.tex]

\appendix
\section{Program Dependence Graphs}
\label{sec:back:pdg}
A program dependence graph (PDG)~\cite{ferrante1987program} consists of the data dependence
graph (DDG) and the control dependence
graph (CDG), whose edges are representing data and control dependencies, respectively.
% We adopt the definitions of DDG and CDG in the original paper~\cite{ferrante1987program}.

\begin{definition}[Data Dependence Graph]
\label{def:ddg}
Given a data dependence graph $DDG(N,E)$, each node in $N$ represents
statements and predicate expressions (or instructions) of the program,
while each edge in $E$ represents a data dependency between two nodes
in $N$. 
One node $n_1 \in N$ is data-dependent on another node $n_0 \in N$,
iff. there is a variable $v$ that is defined at $n_0$ and
used at $n_1$ and there exists a path of nonzero length from $n_0$ to
$n_1$ along which $v$ is not re-defined. 
Then, $(n_0,n_1)$ is a directed edge in $E$.
\autoref{fig:ddg_example} shows the data dependence graph of the
function \cc{setup\_env} in \autoref{code:bit}.
\end{definition} 

\begin{definition}[Control Dependence Graph]
\label{def:cdg} 
Given a control dependence graph $CDG(N,E)$, each nodes in $N$
represent statements and predicate expressions (or instructions) of
the program, while each edge in $E$ represents a control dependency
between two nodes in $N$.
One node $n_1 \in N$ is control-dependent on another $n_0 \in N$ if
and only if $n_0$ is not strictly post-dominated by $n_1$; there
exists a path from $n_0$ to $n_1$ and every node in the path other
than $n_0$ and $n_1$ is post-dominated by $n_1$. 
Then, $(n_0,n_1)$ is a directed edge in $E$.
The CDG of \cc{setup\_env} is shown in \autoref{fig:cdg_example}. 
\end{definition}

\newcommand*\circled[1]{\tikz[baseline=(char.base)]{
            \node[shape=circle,draw,inner sep=0.8pt] (char) {#1};}}
\begin{figure}[t]
    \centering
    \begin{subfigure}[t]{0.49\columnwidth}
    \includegraphics[width=0.6\textwidth]{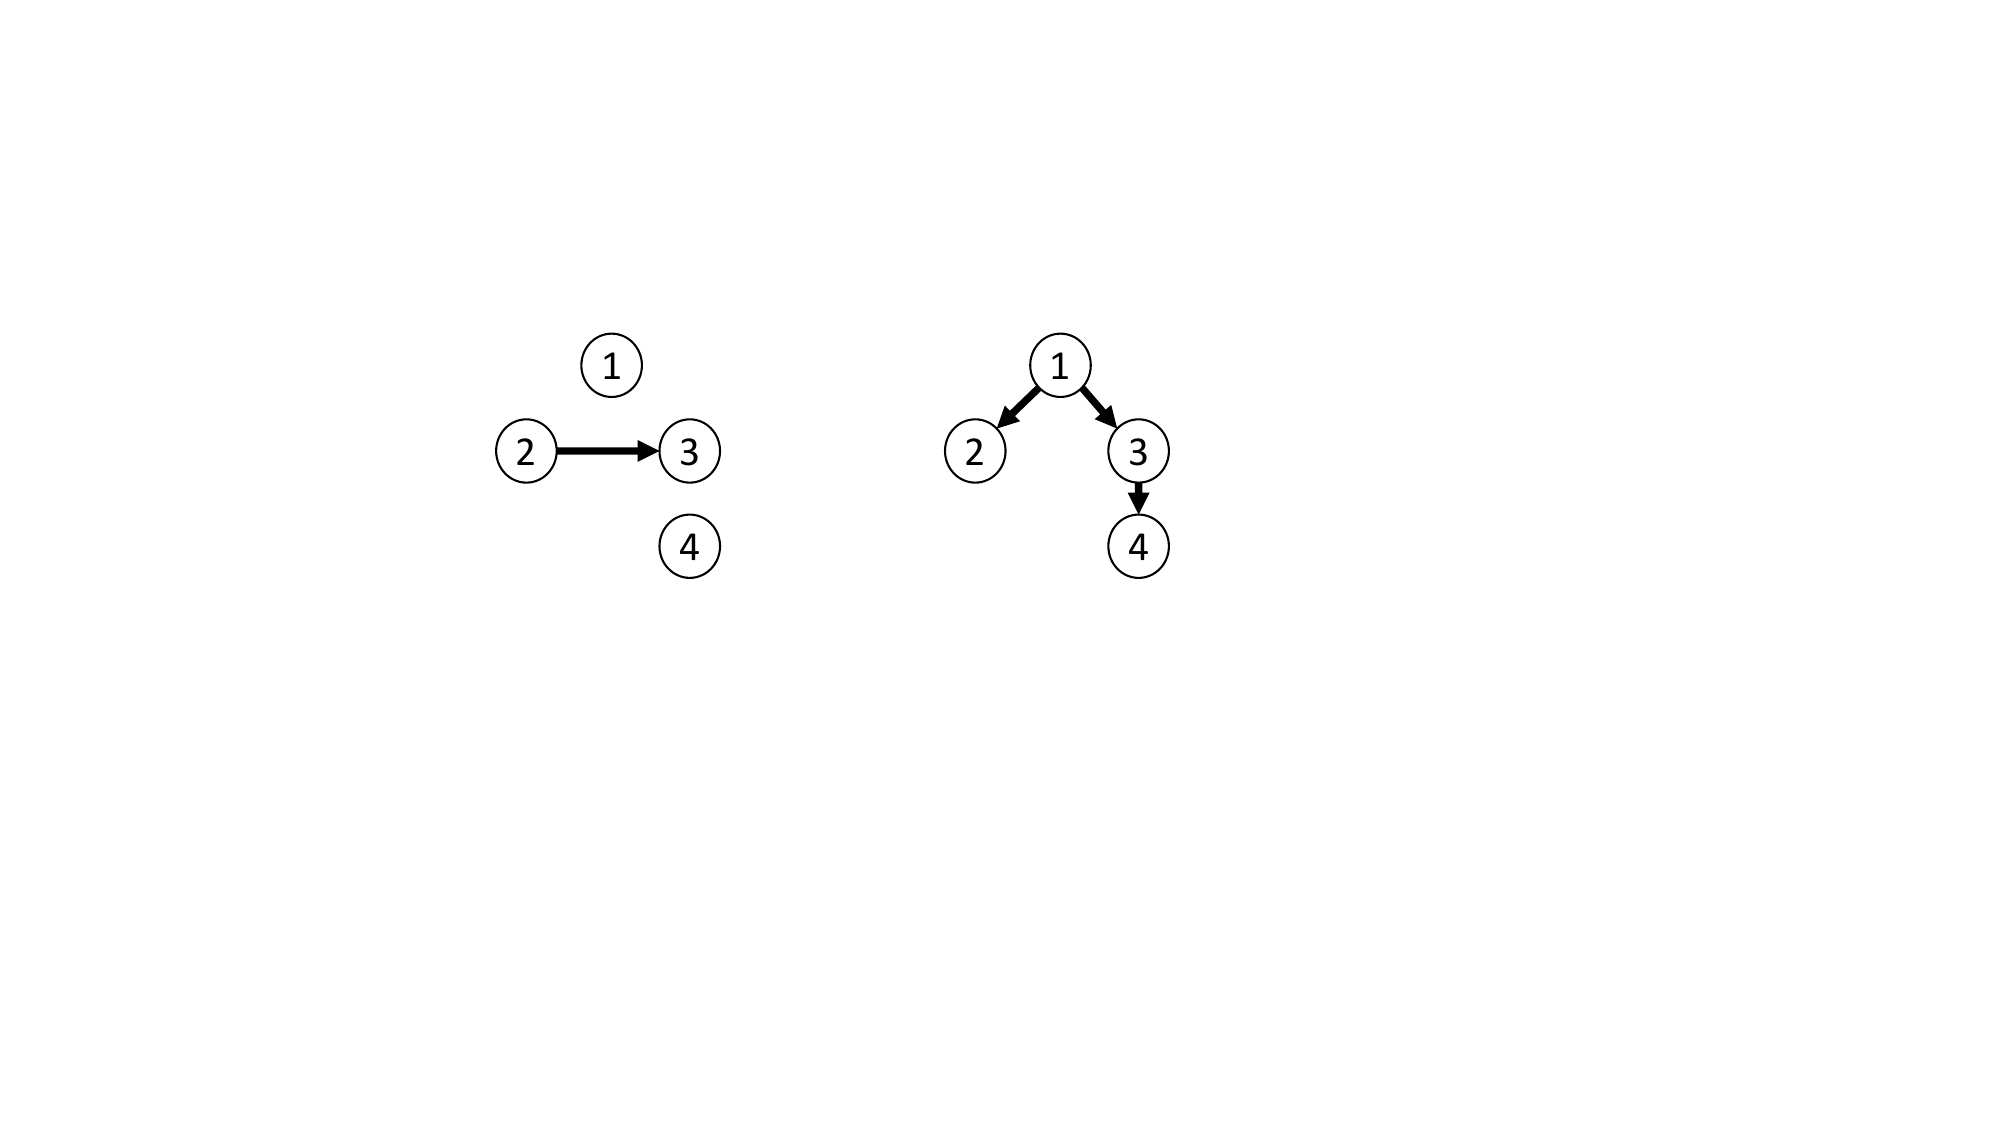}
      \caption{\footnotesize Control Dependence Graph}
      \label{fig:cdg_example}
    \end{subfigure}
    \begin{subfigure}[t]{0.49\columnwidth}
    \includegraphics[width=0.6\linewidth]{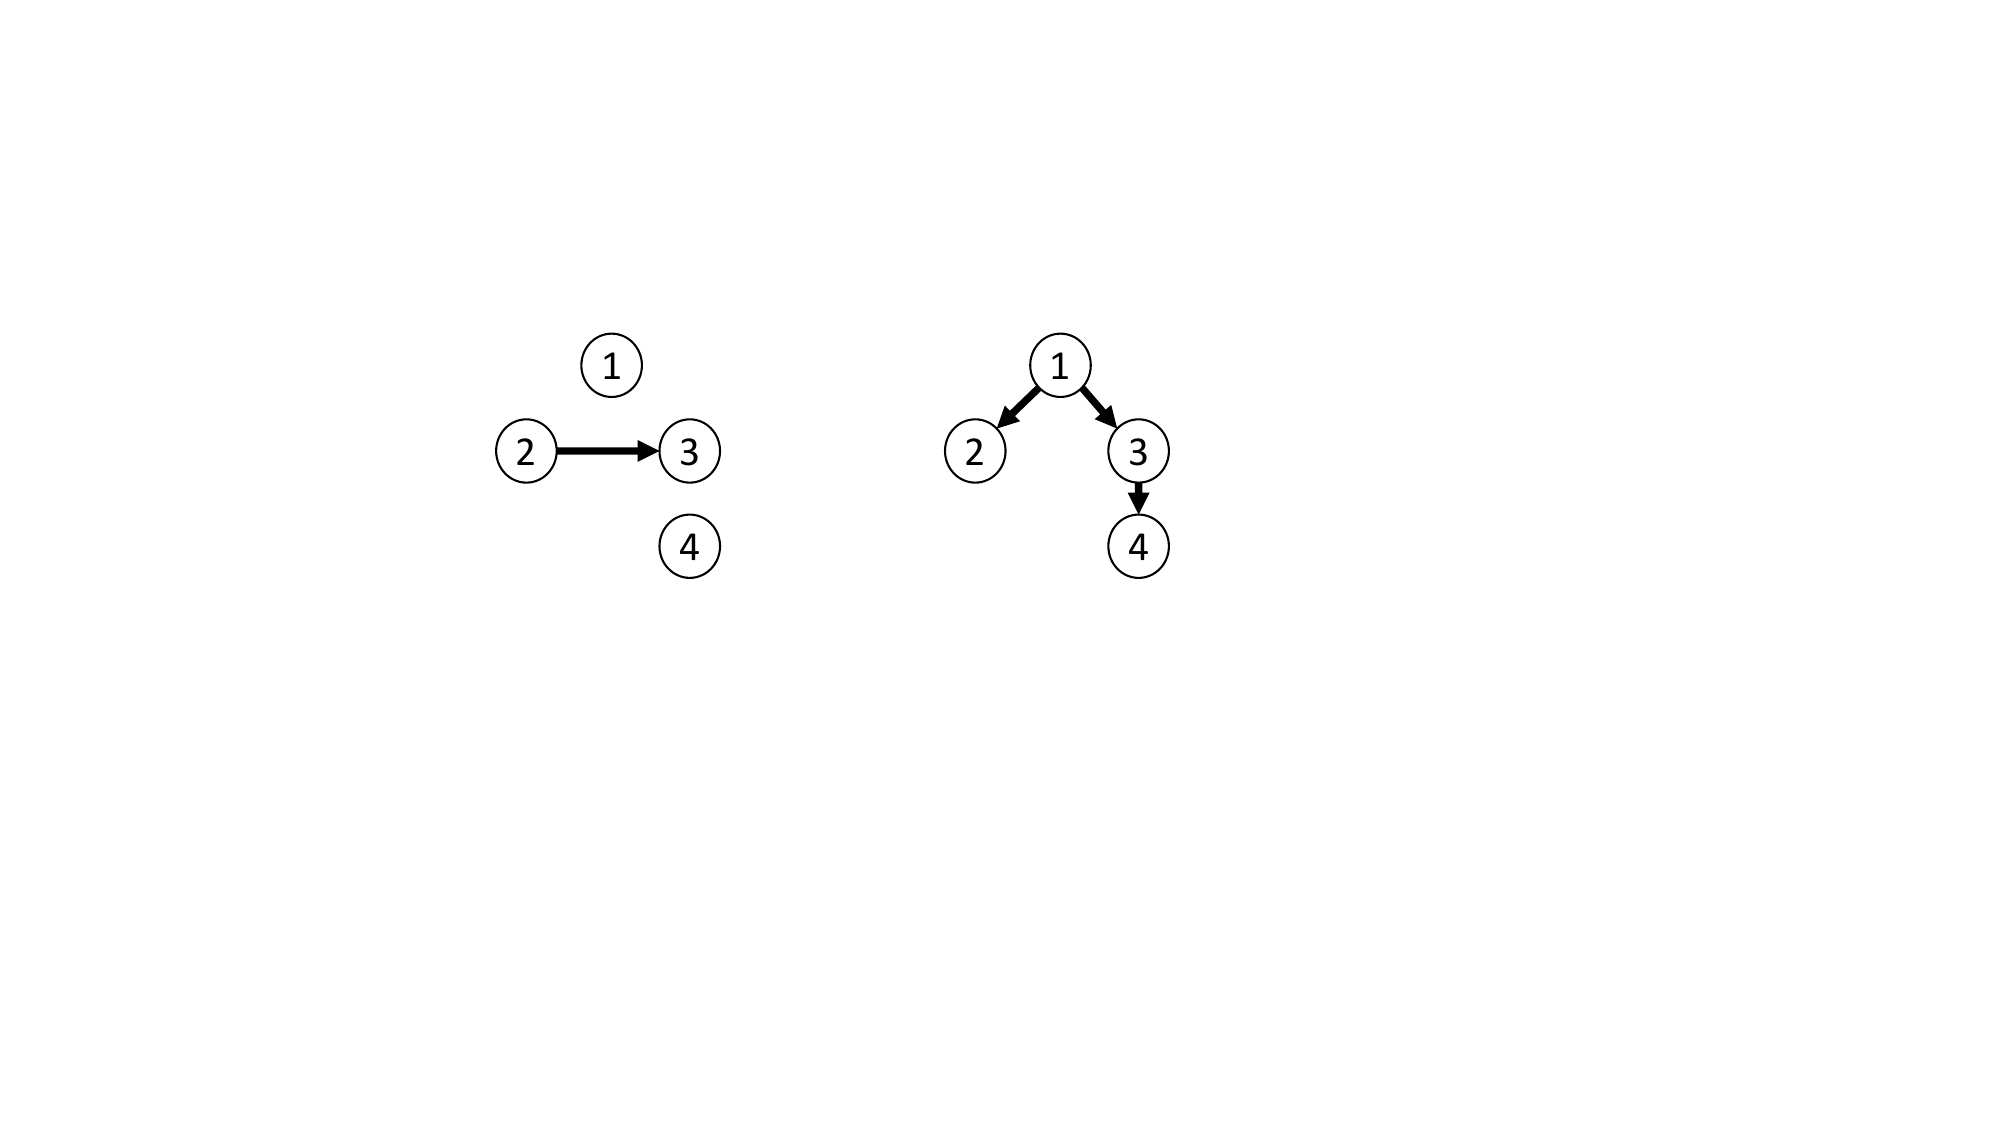}
      \caption{\footnotesize Data Dependence Graph}
      \label{fig:ddg_example}
    \end{subfigure}
    \caption{\footnotesize PDG for function \cc{setup\_env}. {\protect\circled{\scriptsize 1}} {\protect\circled{\scriptsize 2}} {\protect\circled{\scriptsize 3}} and {\protect\circled{\scriptsize 4}} represent statements in line~1, 2, 3, and 4 in \autoref{code:bit}, respectively.}
    \label{fig:pdg_example}
    % \vspace*{-4mm}
\end{figure}

\section{Details of PDG construction}
\label{sec:apdx:graph}
% The runtime analyzer is implemented based on Intel Pin, which builds DFG+ along with program’s execution. Intel Pin provides comprehensive APIs for code inspection and instrumentation: the inspection APIs helps to analyze instructions in binary and the code instrumentation APIs help to instrument code according to the results of inspection. The developed runtime analyzer consists of three components: dynamic code analysis and instrumentation, memory layout restoration, and graph construction. Fig. 3 demonstrates the whole workflow.
To build dynamic PDG for each triggered variables from execution trace, there are two challenges: 1) how to track the liveness of variables. 2) how to obtain the ground truth of each variables, which are labeled by our human experts.
Therefore, we post the technique details here. 
\subsection{Variable liveness analysis}
\label{appdx:live}
% Then, we analyze the execution trace offline to
% track the liveness of variables.
%
1) The liveness of \textbf{global variable} is straightforward and
does not need further analysis.
2) For \textbf{stack variables}, we use the stack allocation at function entry
and deallocation at function exit to indicate their lifetime.
3) For \textbf{heap variables}, we track the memory allocation
(\eg, using \cc{malloc}) and
deallocation (\eg, using \cc{free})
by hooking all heap management functions.
Whenever a stack frame or a heap chunk is deallocated,
we mark the freed region
so that future accesses to this region create new variables.

\subsection{Passing label from source code to binary}
\label{appdx:passing}
There are several ways to
pass the variable labels from the source code to the binary.
In our implementation,
we adopt LLVM pass to insert some redundant instructions (\ie, a special \texttt{prefetch} instruction)
that encode variable labels to target executables during compiling.
% Value *PrefetchFunc = Intrinsic::getDeclaration(Ins->getModule(), Intrinsic::prefetch);
% Instruction* head = OIRB.CreateCall(PrefetchFunc, {con_var_addr, ConstantInt::get(OIRB getInt32Ty(), 0), ConstantInt::get(OIRB.getInt32Ty(), 1), ConstantInt::get(OIRB.getInt32Ty(), 1)});
%
Technically, our LLVM pass will read the ground truth of each variables that our experts labeled, and emit \texttt{prefetch} instructions (though call to \texttt{Intrinsic::prefetch}) which encode the information related to the variables.
For example, following two instructions are emitted when a 4-byte critical variable is allocated at \texttt{0x55555555}.
\begin{center}
  \label{prefetchcritical}
  \vspace*{-0.6em}
  \texttt{prefetcht1 0x55555555}; \\
  \texttt{prefetchnta 0x4};~~~~~~~~~~~~
   \vspace*{-0.6em}
\end{center}
For another example, following two instructions are emitted when a 8-byte non-critical variable is allocated at \texttt{0x66666666}.
\begin{center}
  \label{prefetchnoncritical}
  % \small
  \vspace*{-0.6em}
  \texttt{prefetcht2 0x66666666}; \\
  \texttt{prefetchnta 0x8};~~~~~~~~~~~~
   \vspace*{-0.6em}
\end{center}
The dynamic tracer can know the type (critical or non-critical), address, and length of a variable whenever encountering a pair of such \texttt{prefetch} instruction. 
We adopt the \texttt{prefetch} to pass the information because they do not have any side effects to the program's execution.
When building PDG from the execution trace, we identify and remove these \texttt{prefetch} instructions
from the execution trace, in order to avoid introducing extra code patterns
of critical variables.

\section{Detail of data labeling} 
\label{apdx:label}
\mypara{Background of Human Experts}
To guarantee the quality of data labeling, we invite 2 experts that have more than 6 years experience in data-oriented attack and program analysis, to help us label the data. One of the experts have publish high quality papers on the related topics. 

However, significant amount of human effort is still needed to label critical data, mainly due to its rareness. Therefore, we firstly develop several heuristic-based rules to assist critical-data labeling. These rules conservatively pinpoint candidate variables with a lot of false positives, which will then rely on human analysis to remove.
% Experts manually check the context to confirm the criticalness.

% \mypara{Manual Critical-data Confirmation} 
Once the heuristic-based method
provides a set of candidate critical data,
we rely on human efforts to confirm each of them.
In particular, we consider three concrete attacking scenarios that use critical variables.
First, a variable is useful to grant attackers extra privileges,
such as authentication flags and security configurations~\cite{safemode}.
\autoref{code:bit} illustrated in \autoref{sec:intro} is a typical case of such variables.
Second, a variable enable attackers to bypass authentication by simply modifying it.
Third, an attacker can obtain more permission by control a variable. Specifically, ``more permission'' could mean that attacker can access more files/folders or other useful information. 
If one candidate does not belong to either of two cases,
we label it as a negative sample (\ie, non-critical data). 
A variable will be added into our dataset only when 3 experts agree that it is a critical or non-critical. Otherwise, it exclude from our dataset. 
This dataset took roughly 200 hours labor to generate. The most time-consuming tasks are manual program logic investigation. We tried our best to increase the diversity: \autoref{tab:datacategories} shows the percentage of each category.

\subsection{Case study}
\label{sec:case}

In this section, we conduct case studies to provide our insights about the model decisions. Note that all the statements made in this section are not general conclusions.

%\subsection{True Positive and True Negative Cases}

\mypara{True Positive}
We first start with the model's successes. 
Our model correctly classified the examples shown in the introduction as positive examples. 
As explained in the introduction section, variable {\tt aclp} will carry the information about whether the user is blocked, 
and an attacker can illegally login if the value of the variable is modified during the execution. 
The dependence tree contains the information of the critical operation shown in Code 2, 
and our trained model is able to capture that information. 
% (\hypertarget{evidence1}{\hyperlink{observation1}{\textbf{E1}}}:) 
% Note that the \autoref{fig:dfg-tree} does not show the complete long dependence tree, which contains a good amount of information. 
For example, the opcode feature shows that there are several data transfer operations (\cc{MOV} instructions) and several logical operations. 
% Although not shown in the \autoref{fig:dfg-tree}, 
% there is also a vector operation opcode. 
The number of dominated BBs is also fairly big, which results in 67 changed executed BBs. 
Though it is not possible to completely explain a deep learning model's decision, 
it is clear that the information is rich in this example, and heuristically, 
a variable that is processed by diverse opcodes and with many control dependencies is likely to be critical. 
% \zl{more specific. We can talk about the 1) mov instruction. We can talk about 2) logical operation, 3) bb\_diff, 4) fake the bb\_diff and see the result. } 

% \begin{figure}[!htbp]
%   % \setlength{\belowcaptionskip}{-13pt}
%   \centering
%   \includegraphics[width=0.45\textwidth]{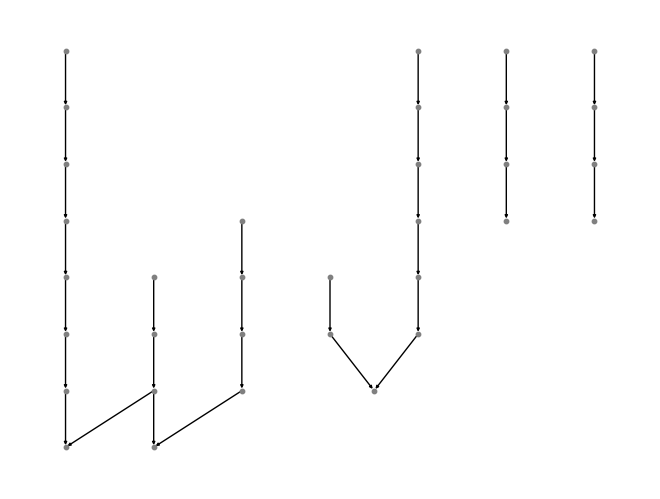}
%   \caption{The Structure of the Data Flow Tree of \autoref{code:bit}.}
%   \label{fig:cs_tp}
% \end{figure}

\mypara{True Negative}
We also discuss an example that the model correctly identifies non-critical data.
The variable \cc{daemonmode} in {\tt bftpd-5.6} controls 
whether the server should be run as a daemon or not.
% which is very unlikely to be interested by an attacker. 
% Even if an attacker manages to modify it, 
% the server maintainer will immediately realize that the program is not running as expected. 
With careful checks, 
we believe this variable is non-critical
as the program behavior is almost the same
regardless whether the program is running as daemon or not.
The use of this variable is quite simple: 
it is initialized with a value from the command line 
or the configuration file, and 
then gets checked during the program setup
before spawning the daemon. 
These uses result in three dependence trees are partially shown in \autoref{fig:cs_abs} (a). 
The dependency paths in these tree are short and no fork is presented. 
% Although one can observe the CMP operations, 
% it is not likely a critical variable to have such short data flow. 
% For example, 
% an authentication flag will have a more complicated data flow, 
% as the program will need to check many conditions. 
In addition, the number of dominated BBs is only 1, 
which means that the only few basic block control dependent on it.
% executed basic blocks are only changed by 1
% when it is flipped.
%
% We believe this is the main reason that
% our model classifies this variable as non-critical.
% \haizhou{For every case, we mention 4 things: 1) straight lines, 2) logical operation, 3) bb\_diff, 4) not very long (simple dfg)}

% \begin{figure}[!htbp]
%   % \setlength{\belowcaptionskip}{-13pt}
%   \centering
%   \includegraphics[width=0.45\textwidth]{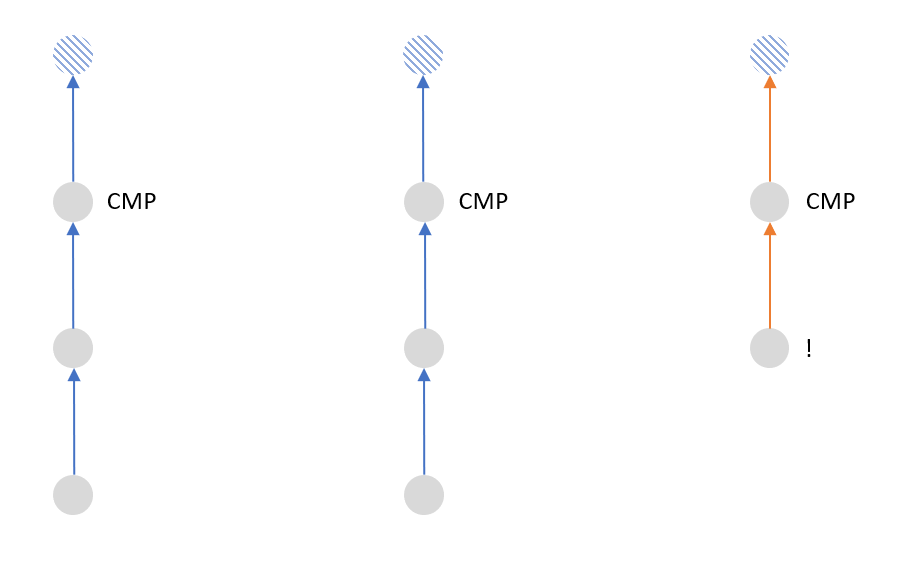}
%   \caption{The Data Flow Tree of Variable {\tt daemonmode}.}
%   \label{fig:cs_tn}
% \end{figure}

%% Next, we take a close look at the model's failures: another two examples from {\tt bftpd-5.6}. 

\begin{figure}[t]
  \centering
  \includegraphics[width=0.38\textwidth]{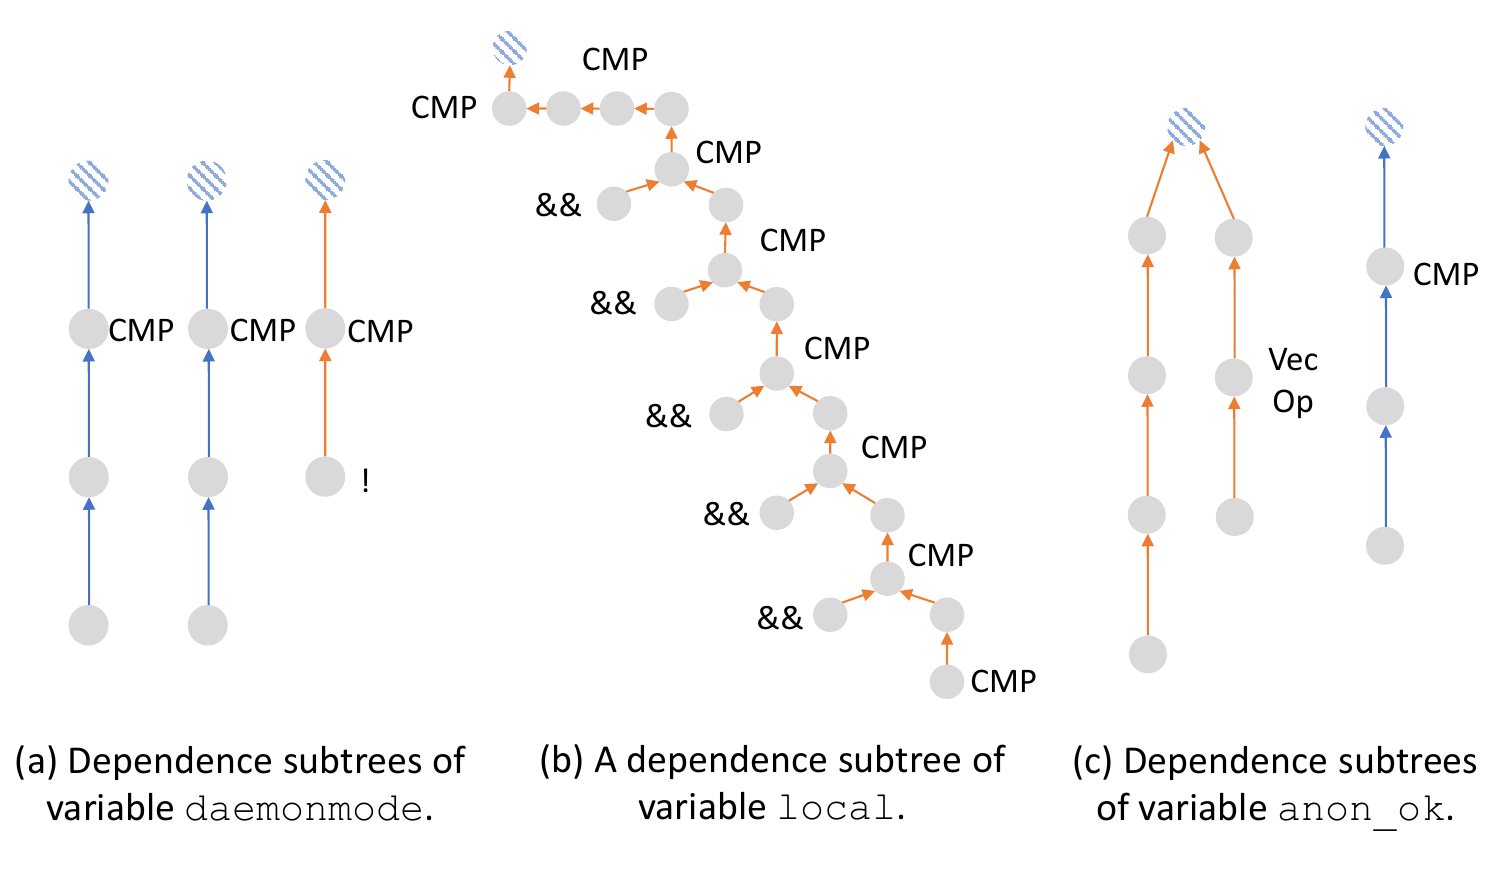}
  \caption{\textbf{Dependence subtrees for case studies.}}
  \label{fig:cs_abs}
\end{figure}

\mypara{False Positive} 
In this example, our model incorrectly classifies one non-critical variable as critical.
Specifically, variable {\tt local} is used in \cc{bftpd-5.6} to 
find the timezone difference between a client and the server, 
only for security-unrelated operations such as logging.
But our model gives the unexpected label. 
By checking its dependence trees partially shown in \autoref{fig:cs_abs} (b), 
we found that the dependencies are complicated,
including many comparison and logical operations to compare two time zones,
% as finding a time zone difference involves many comparisons. 
%%Further more, there are many branches in the data-flow tree, 
%which implies the value of the variable is not acquire in a straight forward manner. 
%This observation is usually related to the critical flags. 
The number of dominated BBs is 5, 
indicating this variable can slightly influence 
the overall program execution. 
All these facts confuse our model to draw 
the wrong conclusion. 
A human analyst can filter this variable out 
when figuring out that it is not related to security-related operations. 
However, at binary level no comment or name information in the traces can be used.

\mypara{False Negative}
Lastly, we examine a case where the model misses a critical variable. 
{\tt anon\_ok} is a flag indicating whether anonymous logins are allowed. 
By modifying this flag, attackers can anonymously login to the server,
and then conduct illegal access or launch deny-of-service attacks.
%so many administrators will disable this functionality. 
% Therefore, this variable should be considered as critical. 
\autoref{fig:cs_abs} (c) shows its full define-flow tree (left) and use-flow tree (right).
The define-flow tree has a vector operation,
and the use-flow tree contains a \cc{CMP} operation.
The whole paths of dependencies are fairly short,
and the number of dominated BBs is only 17, which could indicate that 
this variable is not very critical. 
%This data could be critical 
%when it is encryption-related data, 
%but encryption-related data usually has unique data-flow pattern, 
%and the model does not think this is the case. 
%
The reason for this misclassification is similar to the false positive case. 
When a human analyst looks at the variable, 
it is obvious that the data is related to anonymous login and thus critical,
but the model does not have access to this information.

\section{Runtime overhead of our tool-chain}
\label{apdx:time}
\begin{table}[t]
  \captionsetup{justification=centering}
    \caption{\textbf{Performance evaluation,} including time and memory consumption of tracing, graph construction, and model inference.}
    \label{tab:run}
    \centering
    \footnotesize
    \setlength{\tabcolsep}{5pt}
    \begin{tabular}{lllll}
    \toprule
    \multirow{2}{*}{\bf Program} &
    \multicolumn{1}{l}{\bf Tracing} &
    \multicolumn{2}{l}{\bf Graph Construction}&
    \multicolumn{1}{l}{\bf Inference} \\
    \cline{3-4}
       & Time (s)  & Trace Size(Ins) & Time(m\&s)  &  Time(s)/Per-Var \\
    \midrule
    nginx  &	12.4 & 3059335  & 47.11s  &  0.3129  \\ %  126.7392 / 405
    %\hline
    % vsftpd  & 5.1 & 986613   & 15.26   & 167 & 20.58 & \\
    % \hline
    bftpd & 23.5  & 85519298  & 12m38.476s    & 0.1304 \\ % 11.3483/ 87
    %\hline
    proftpd  & 45.1  & 130065689  & 19m52.295s    & 0.4077\\ % 113.3326 / 278
    %\hline
    ghttpd & 3.1  & 600177  & 9.704s    & 0.1247 \\ %  5.2369 (s) / 42
    %\hline
    % telnetd  & 16.4  & 12269a  & 7.963s   & 167 & 20.58 & \\
    % \hline
    telnet  & 20.58  & 514522  & 8.579s  &  0.1697 \\ % 6.4475 / 38
    %\hline
    vsftpd  & 20.58  & 986613  & 15.176s   & 0.2426 \\ % 200.180 (s) / 825
    \bottomrule
    \end{tabular}
    % \vspace*{-3mm}
  \end{table}

  \autoref{tab:run} shows the measured times consumed to trace, build each PDG, and %the average time consumed by the DL model 
  produce a prediction, respectively. 
  We note that it takes only 0.12-0.41 seconds 
  to produce one prediction. 
  In addition, building PDGs from 
  execution traces is the most time-consuming step. 
  Nevertheless, even for a fairly large program such as \cc{proftpd}, our
  tool can build PDGs for all the triggered variables within 20 minutes. 
  Since it takes more time for human analysts to review 
  the predicted variables,  
  our tool-chain provides reasonable time efficiency. 

{\bf Model size and training time. }
The size of our Tree-LSTM model is 2,194 (\ie, \# of parameters), while the size of RGCN is 7,218.
The size of our model, which is more accurate, is substantially smaller than RGCN. 
In terms of training time, the average per-epoch time is 1,029 seconds for RGCN and 521 seconds for our model, respectively.  

\begin{table*}[t]
  \captionsetup{justification=centering}
\caption{\textbf{Newly uncovered critical variables that were confirmed by GDB.} }
\label{tab:gdbconfirm}
\centering
\footnotesize
\setlength{\tabcolsep}{4pt}
%\begin{tabular}{m{0.8cm}<{\centering}|m{0.6cm}<{\centering}|m{0.6cm}<{\centering}|m{0.7cm}<{\centering}|m{0.6cm}<{\centering}|m{0.6cm}<{\centering}|m{0.6cm}<{\centering}|c}
\begin{tabular}{m{2.8cm}<{}m{3.8cm}<{}m{2.5cm}<{}m{3.8cm}<{}m{3cm}<{}}
\toprule
{\bf Program} & {\bf Function} & {\bf Variable}  & {\bf The Potential Attack} & {\bf GDB Break Point}  \\
\midrule
php\_php-fuzz-parser  &  \texttt{zend\_disable\_functions}  &  function\_list  &  permission escalation & zend\_API.c:3263 \\
php\_php-fuzz-parser & \texttt{virtual\_cwd\_main\_cwd\_init} & cwd & changing work directory  & zend\_virtual\_cwd.c:188 \\
% mbedtls\_fuzz\_dtlsclient  &  \texttt{rsa\_rsassa\_pkcs1\_v15\_encode}  &  nb\_pad  &  Bleichenbacher's forgery attack~\cite{izu2007analysis} & rsa.c:1761 \\
nginx  &  \texttt{ngx\_process\_options}  &  cycle-confix.data &  config manipulation & nginx.c:987 \\
curl\_curl\_fuzzer\_http  &  \texttt{seturl}  &  path &  URL manipulation  & urlapi.c:852 \\
sqlite3\_ossfuzz &  \texttt{appendAllPathElements}  &  pPath->zOut &  config manipulation  & sqlite3.c:42001 \\
sqlite3\_ossfuzz &  \texttt{sqlite3BtreeEnter}  &  p->sharable &  permission escalation  & sqlite3.c:66648 \\
sqlite3\_ossfuzz &  \texttt{sqlite3TableLock}  &  iDb &  permission escalation  & sqlite3.c:115275 \\
% Sqlite3  &  \texttt{decodeNumber}  &  rc &  permission escalation attack  & json\_reader.cpp:562 \\
% jsoncpp\_jsoncpp\_fuzzer  &  \texttt{decodeNumber}  &  threshold &  integer overflow attack  & json\_reader.cpp:562 \\
\bottomrule
\end{tabular}
%\vspace{-1em}
\end{table*}
\section{Did the model learn the ``implicit patterns''?}
\label{apdx:implicit}

%We mentioned that we need to exploit ``implicite patterns'' to accurately identify critical data in~\autoref{sec:intro}. 
To demonstrate that ``explicit patterns'' usually don't exist, we adopt t-SNE~\cite{van2008visualizing} to visualize the data points.
t-SNE~\cite{van2008visualizing} is a technique to visualize high-dimensional data by giving each data point a location in a two or three-dimensional map.
\autoref{fig:tsne} are visualizations of the raw feature embedding and the representation learned by our model, respectively. Blue and red points represent critical and noncritical variables, respectively, whereas different types of shapes represent different programs. 
\autoref{fig:tsne} (a) shows that there is no explicit pattern that can distinguish the critical and noncritical variables based on the raw feature embeddings. 
\autoref{fig:tsne} (b) shows that a combination of dependency tree and Tree-LSTM is able to map the data points to another feature space, which enables ``implicit patterns'' to %pinpoint the critical variables.
create a distance between the clusters of critical variables 
and the clusters of non-critical variables. 

\begin{figure*}[t]
  \centering
  \includegraphics[width=\columnwidth]{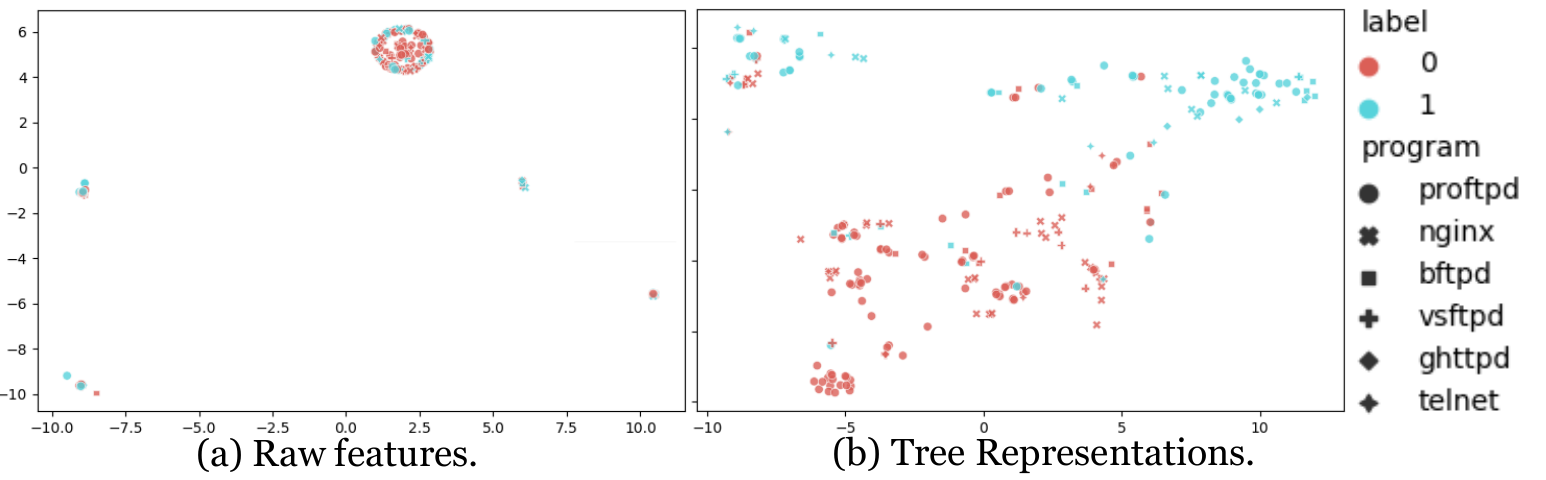}
  \caption{t-SNE visualisation of the tree representations, and raw feature embeddings.}
  \label{fig:tsne}
  % \vspace*{-2mm}
\end{figure*}

\section{Details of GDB confirmed critical data} 
\label{sec:appdx:gdb}

Let's take a closer look at the six involved programs in~\autoref{tab:gdbconfirm}:   
{\bf php:} The details of \texttt{disabled\_functions} has been shown \autoref{sec:intro} based on \autoref{code:php}.
\sout{in allows one to disable certain functions, whose name are read from the configuration file (php.ini). By modifying this variable, attacker can remove the security-critical functions, such as \texttt{exec()}, \texttt{shell\_exec()}, \texttt{curl\_exec()}) from the blocked list and then invoke them to execute malicious behaviors.}
\texttt{cwd} in \texttt{virtual\_cwd\_main\_cwd\_init} holds the path of working directory, which can be used to access other folders by modifying this variable. 
% {\bf mbedtls:} In function \texttt{rsa\_rsassa\_pkcs1\_v15\_encode()}, there is a static boundary check (\cc{nb\_pad < 10 + hashlen + oid\_size}) to prevent Bleichenbacher's forgery attack against lax PKCS\#1v1.5 verification~\cite{izu2007analysis}. Modifying the variable \cc{nb\_pad} enable the attackers to launch the Bleichenbacher's forgery attack. 
{\bf nginx:} \texttt{cycle-confix.data} temporarily holds the path of configuration file that will be processed by \texttt{ngx\_process\_options}.
{\bf curl:} Variable \texttt{path} holds the location of the data that \texttt{curl} will transfer. By modifying \texttt{path}, attacker can transfer data from an unexpected location, or transfer a malicious file. 
{\bf sqlite3:}  
% we will introduce 1 out of 3 in sqlite3 due to page limited. sqlite3 
Variable \texttt{pPath->zOut} holds the location of an opened database; 
variable \texttt{p->sharable} controls if a pBt can be shared with another database. 
Modifying \texttt{iDb} can bypass a lock to a database table.

%------------------
\section{Detailed of critical variable found in other types of programs}
\autoref{tab:newdetails} list all the found potential critical variables in \texttt{curl}, \texttt{php}, and \texttt{sqlite3}.
\onecolumn
\begin{center}[!]
  \scriptsize
  \begin{ThreePartTable}
    \begin{TableNotes}
    \footnotesize
    \item[1] a brief explanation why the variable is potentially critical based on a quick analysis.
    \item[2] the filename and line number.
    \end{TableNotes}
  \begin{longtable}{p{0.1cm}<{\centering}p{2cm}<{}p{2cm}<{}p{2cm}<{}p{5.8cm}<{}}
  \caption{Found potential critical variables in FuzzBench programs by our tool.} \label{tab:newdetails} \\
  % Function & Variable  & Location~\tnote{1}  & Label~\tnote{2}  & Explain~\tnote{3}\\
  \hline \hline
   \multicolumn{1}{c}{\bf{Program}} & \multicolumn{3}{l}{\bf{Name of}} & \multicolumn{1}{l}{\bf{Brief Description}~\tnote{1}} \\ 
   \cline{2-4}
   & \multicolumn{3}{l}{\bf{Func} \& \bf{Var} \& \bf{File}~\tnote{2}} & \\
    \hline 
  \endfirsthead
  
  \multicolumn{5}{c}%
  {{\bfseries \tablename\ \thetable{} -- continued from previous page}} \\
  \hline \hline
  \multirow{2}{*}{\bf{Program}} & \multicolumn{3}{l}{\bf{Name of}} & \multicolumn{1}{c}{\bf{Brief Description}~\tnote{1}} \\ 
  \cline{2-4}
  %  & {\bf{\emph{Func}}} & {\bf{\emph{Var}}} & {\bf{\emph{File}}~\tnote{2}} & \\ 
  & \multicolumn{3}{l}{\bf{Func} \& \bf{Var} \& \bf{File}~\tnote{2}} & \\
   \hline 
  \endhead
  
  \hline \multicolumn{5}{r}{{Continued on next page}} \\ \hline
  \endfoot
  \hline \hline
  \insertTableNotes
  \endlastfoot
  \hline
  \multirow{2}{*}{\bf curl} & \multicolumn{3}{l}{seturl \& path \& urlapi.c:852} & the url link to requested resource \\ %
  & \multicolumn{3}{l}{getparameter \& hit \& tool\_getparam.c:596}   & config parser \\ % 
  &  \multicolumn{3}{l}{curl\_multi\_add\_handle \& dns.hostcachetype \& multi.c:514}   & dns cache \\ %  
   &  \multicolumn{3}{l}{main\_init \& result \& tool\_main.c:166}   & control config initialise\\ %  
  &  \multicolumn{3}{l}{findfile \& fname \& tool\_findfile.c:107}   & related to ".ssh/known\_hosts \\ %"
  &  \multicolumn{3}{l}{operate \& result \& tool\_operate.c:2636}   & control parsing of command line arguments  \\ %"
  &  \multicolumn{3}{l}{operate \& res \& tool\_operate.c:2609}   & control parsing of command line arguments  \\ %"
  &  \multicolumn{3}{l}{Curl\_vsetopt \& version\_max \& setopt.c:416}   & restrict to the version SSL to connect \\ %"
  &  \multicolumn{3}{l}{findfile \& fname \& tool\_findfile.c:107}   & get the path of file to open \\ 
  &  \multicolumn{3}{l}{operate \& argc \& tool\_operate.c:2588}   & number of arguments to parse \\ 
  &  \multicolumn{3}{l}{curl\_share\_setopt \& share \& share.c:62}   & control resource sharing \\ 
  %  & multi\_runsingle & data & multi.c:1777   & related to connection control \\
  %  & Curl\_vsetopt & set-\textgreater{}magic & setopt.c:2218   & related to global variable mutexing \\ %file descriptor for file in homedir, specifically .ssh/known\_hosts
  &  \multicolumn{3}{l}{Curl\_vsetopt \& set \& setopt.c:2218}   & related to global variable mutexing \\ 
  &  \multicolumn{3}{l}{checkhome \& c \& tool\_findfile.c:78}   & check the home dir \\
  &  \multicolumn{3}{l}{Curl\_is\_absolute\_url \& i \& urlapi.c:251}   & related the url link to requested resource \\
   &  \multicolumn{3}{l}{single\_transfer \& global \& tool\_operate.c:806}   & config to control program behavir \\
   &  \multicolumn{3}{l}{Curl\_pretransfer \& result \& transfer.c:1492}   & control constraints checking\\ % control Recheck all uniqueness constraints after replace triggers have run
   &  \multicolumn{3}{l}{easy\_transfer \& mcode \& easy.c:598}   & state variable \\
   &  \multicolumn{3}{l}{Curl\_init\_userdefined \& result \& url.c:596}   & state variable \\
   &  \multicolumn{3}{l}{curl\_easy\_init \& initialized \& easy.c:288}   &  flag to control SSL \\ %flag to denote whether global SSL stuff is initialized
  \hline
  \multirow{2}{*}{\bf php}  &  \multicolumn{3}{l}{zend\_disable\_functions  \& function\_list \& zend\_API.c:3263}    & block call to critical functions such as \texttt{execv()}  \\
   &  \multicolumn{3}{l}{virtual\_cwd\_main\_cwd\_init \& cwd \& zend\_virtual\_cwd.c:180}   &  current working directory \\
   &  \multicolumn{3}{l}{alloc\_globals\_ctor \& tmp \& zend\_alloc.c:2877}   & environment variable \\
   &  \multicolumn{3}{l}{php\_output\_set\_implicit\_flush \& flush \& output.c:750}   & connection timeout \\
   &  \multicolumn{3}{l}{zend\_cpu\_startup \& cpuinfo.initialized \& zend\_cpuinfo.c:116}   & control the cpu resource \\
   &  \multicolumn{3}{l}{zend\_add\_system\_entropy \& finalized \& zend\_system\_id.c:31}   & control system entropy \\
   &  \multicolumn{3}{l}{tsrm\_realpath \& path \& zend\_virtual\_cwd.c:1716}   &  current work dir \\
   &  \multicolumn{3}{l}{zend\_set\_timeout\_ex \& seconds \& zend\_execute\_API.c:1454}   & seconds of the timeout \\
   &  \multicolumn{3}{l}{php\_init\_config \& php\_ini\_scanned\_path \& php\_ini.c:642}   &  configuration file path \\
   &  \multicolumn{3}{l}{save\_ps\_args \& i \& ps\_title.c:165}   & index of arguments in argument parser \\
   &  \multicolumn{3}{l}{zend\_register\_functions \& target\_function\_table \& zend\_API.c:2668}   & registers all functions in library\_functions \\
   &  \multicolumn{3}{l}{zend\_register\_functions \& type \& zend\_API.c:2662}   & control the type of registered function (USER\_FUNCTION/INTERNAL\_FUNCTION) \\
   &  \multicolumn{3}{l}{zend\_unregister\_ini\_entries\_ex \& module\_type \& zend\_ini.c:281}   & control unregister of function \\
   &  \multicolumn{3}{l}{tsrm\_realpath\_r \& save \& zend\_virtual\_cwd.c:952}   & flag to choose directories \\
   &  \multicolumn{3}{l}{sapi\_header\_op \& op \& SAPI.c:710}   & specify the type of operation \\
   &  \multicolumn{3}{l}{zend\_func\_info\_shutdown \& zend\_func\_info\_rid \& zend\_func\_info.c:228}   & control the removal of functions \\
   &  \multicolumn{3}{l}{zend\_do\_perform\_implementation\_check \& fe\_num\_args \& zend\_inheritance.c:708}   & control implementation check \\
   &  \multicolumn{3}{l}{zend\_objects\_store\_call\_destructors \& objects \& zend\_objects\_API.c:46}   & control the object to destroy \\
   &  \multicolumn{3}{l}{php\_output\_lock\_error \& op \& output.c:779}   & control the check of unallowed operation \\
   &  \multicolumn{3}{l}{zend\_get\_resource\_handle \& last\_resource\_number \& zend\_extensions.c:260}   & control resource allocation \\

  \hline
   \multirow{2}{*}{\bf sqlite3} &  \multicolumn{3}{l}{appendAllPathElements  \&  pPath->zOut \& sqlite3.c:42001}   & conf loading attack   \\
   &  \multicolumn{3}{l}{sqlite3BtreeEnter  \&  p->sharable \& sqlite3.c:66648}   &  permission escalation attack   \\
   &  \multicolumn{3}{l}{sqlite3TableLock \& iDb \& sqlite3.c:115275}   & index of the database containing the table to lock \\
   &  \multicolumn{3}{l}{posixUnlock \& eFileLock \& sqlite3.c:37425}   & file locker \\
   &  \multicolumn{3}{l}{sqlite3ParseObjectReset \& db-\textgreater{}lookaside.bDisable \& sqlite3.c:135122}   & new lookaside allocations are only allowed if bDisable==0 \\
   &  \multicolumn{3}{l}{sqlite3\_initialize \& rc \& sqlite3.c:170948}   & database access permission and status \\
   &  \multicolumn{3}{l}{sqlite3GenerateConstraintChecks \& nReplaceTrig \& sqlite3.c:128698}   & control Recheck all uniqueness constraints after replace triggers have run \\
   &  \multicolumn{3}{l}{verifyDbFile \& buf.st\_nlink \& sqlite3.c:36961}   & check how many thread open the database file \\
   &  \multicolumn{3}{l}{unixAccess \& flags \& sqlite3.c:41899}   & test the existence of or access permissions of file zPath\\
   &  \multicolumn{3}{l}{main \& getenv \& shell.c:23113}   & env of ``SQLITE\_DEBUG\_BREA'' \\
   &  \multicolumn{3}{l}{sqlite3VdbeExec \& i \& sqlite3.c:91823}   & index to zPayload that used to execute VDBE program \\
   &  \multicolumn{3}{l}{sqlite3\_appendvfs\_init \& rc \& shell.c:6708}   & control the registration of a statically linked extension \\
   &  \multicolumn{3}{l}{sqlite3PagerOpen \& pPager->noSync \& sqlite3.c:58923}   & sync control \\
   &  \multicolumn{3}{l}{ftsCompareFunction \& keyClass \& sqlite3.c:184968}   & control choose of hash function \\
   &  \multicolumn{3}{l}{whereLoopAddAll \& hasRightJoin \& sqlite3.c:158228}   & hasRightJoin flag prevent FROM-clause terms from moving from the right to the left side of that join  \\
   &  \multicolumn{3}{l}{sqlite3VdbeLeave \& p->lockMask \& sqlite3.c:82620}   & lock mask  \\
   &  \multicolumn{3}{l}{vdbeCommit \& rc \& sqlite3.c:83657}   & state variable  \\
   &  \multicolumn{3}{l}{sqlite3FinishCoding \& pParse->bReturning \& sqlite3.c:115452}   & parse executable code \\
   &  \multicolumn{3}{l}{setGetterMethod \& pPager \& sqlite3.c:54973}   & control the choose of Getter method \\
   &  \multicolumn{3}{l}{do\_meta\_command  \& nArg  \& shell.c:19874}   & command parser \\
   &  \multicolumn{3}{l}{resolveP2Values  \& p->readOnly  \& sqlite3.c:81541}   & permission control \\
   &  \multicolumn{3}{l}{sqlite3\_finalize  \& v  \& sqlite3.c:86117}   & virtual machine to destroy\\
   &  \multicolumn{3}{l}{unixFileControl  \& pFile  \& sqlite3.c:39521}   &  control of an open file handle  \\
   &  \multicolumn{3}{l}{unixFileControl  \& newLimit  \& sqlite3.c:39516}   &  restrinction to file controler  \\
   &  \multicolumn{3}{l}{sqlite3Select \& sSort.pOrderBy->nExpr  \& sqlite3.c:142854}   &  control the sort order  \\
   &  \multicolumn{3}{l}{pcache1Unpin  \& pGroup->nPurgeable>pGroup->nMaxPage  \& sqlite3.c:53068}   &  page num limits \\
   &  \multicolumn{3}{l}{whereLoopInsert  \& pBuilder->iPlanLimit  \& sqlite3.c:156502}   &  search num limits \\
   &  \multicolumn{3}{l}{sqlite3VdbeReset  \& p  \& sqlite3.c:84120}   &  control reset of VDBE (Virtual Database Engine) \\
   &  \multicolumn{3}{l}{sqlite3Init  \& commit\_internal  \& sqlite3.c:134990}   &  control commit of the change \\
   &  \multicolumn{3}{l}{sqlite3VdbeHalt  \& p  \& sqlite3.c:83923}   &  state variable of the VDBE halting \\
   &  \multicolumn{3}{l}{unixAccess  \& flags  \& sqlite3.c:41899}   &  file access permission flag \\
   &  \multicolumn{3}{l}{process\_input  \& p->inputNesting  \& shell.c:22709}   &  input nesting limits \\
   &  \multicolumn{3}{l}{shell\_exec  \& pArg  \& shell.c:15001}   &  control arg of exec \\
   &  \multicolumn{3}{l}{unixClose  \& pInode->nLock  \& sqlite3.c:37616}   &  file lock \\
   &  \multicolumn{3}{l}{sqlite3\_wal\_autocheckpoint  \& nFrame  \& sqlite3.c:173072}   &  enables/disables automatic checkpoints \\
   &  \multicolumn{3}{l}{sqlite3PagerSharedLock \& rc  \& sqlite3.c:59232}   & state variable to obtain share locker \\
   &  \multicolumn{3}{l}{unixOpen \& randomnessPid  \& sqlite3.c:41632}   & process ID \\
   &  \multicolumn{3}{l}{sqlite3Step \& db->nVdbeActive  \& sqlite3.c:86675}   & VDBE status variable \\
   &  \multicolumn{3}{l}{selectExpander \& p->pEList->nExpr>db->aLimit \& sqlite3.c:141655}   & column limits \\
   &  \multicolumn{3}{l}{posixUnlock \& rc \& sqlite3.c:37530}   & pFile->eFileLock\\
   &  \multicolumn{3}{l}{sqlite3\_finalize  \& v  \& sqlite3.c:86117}   & virtual machine to destroy\\
  \end{longtable}
\end{ThreePartTable}
  \end{center}
